# Supplementary material for: Fishr: Invariant Gradient Variances for Out-of-Distribution Generalization
Source: arXiv:2109.02934 source file (2022-06-01)
Supplement: Supplementary file 1 [file 07_appendix_pseudocode.tex]

% \clearpage
\section{Pseudo code}
\label{appendix:pseudocode}
\begin{algorithm}[H]%
    \DontPrintSemicolon%
    \tcc{Setup}%
    \KwParams{Network $f_{\theta}$, made of a deep features extractor $\Phi_{\phi}$ and a dense linear classifier $w_{\omega}$, randomly initialized.}
    \KwInput{
    Observations $\mathcal{D}_{e}=\left\{\left(\vx_{e}^{i}, \vy_{e}^{i}\right)\right\}_{i=1}^{n_{e}}$ for domains $e\in\mathcal{E}$,
    regularization weight $\lambda$, warmup iteration $i_{\text{warmup}}$ and exponential moving average speed $\gamma$, batch size $b_s$, optimizer $g$, learning rate $l_r$.}%
    \tcc{Training Procedure}%
    Initialize moving averages: $\forall e\in\mathcal{E}, \vv_e^{\text{mean}}\gets 0$\\
    \For{$\text{iter}$ \textbf{from} $1$ \textbf{to} \#iters} {%
    \tcc{Step 1: standard ERM procedure}%

    \For{$e\in\mathcal{E}$} {%
    Randomly select batch: $\{(\vx_{e}^{i}, \vy_{e}^{i})\}_{i\in \mathcal{B}}$ of size $b_s$\\
    Compute predictions: $\forall i\in \mathcal{B}, \hat{\vy}_e^{i} \gets f_{\theta}(\vx_{e}^i)$\\
    Compute domain empirical risk: $\mathcal{R}_{e}(\theta) \gets \sum_{i\in \mathcal{B}} \ell\left(\hat{\vy}_e^{i}, \vy_{e}^{i}\right)$
    }
    $ \mathcal{L}(\theta)=\frac{1}{|\mathcal{E}|} \sum_{e\in\mathcal{E}} \mathcal{R}_{e}(\theta)$\\
    \tcc{Step 2: gradient variances in classifier}
    \For{$e\in\mathcal{E}$} {%
    Compute individual gradients in $w_{\omega}$ with BackPACK: $\forall i\in \mathcal{B}, \vg_{e}^{i} \gets \nabla_{\omega} \ell\left(\hat{\vy}_e^{i}, \vy_{e}^{i}\right)$\\
    Compute domain-level gradient variances:
    $\vv_e^{\text{iter}} = \frac{1}{b_s}\sum_{i\in\mathcal{B}}(\vg_{e}^{i}-\frac{1}{b_s}\sum_{j\in\mathcal{B}} \vg_{e}^{j})^2$\\
    Moving average: $\vv_e \gets \gamma \vv_e^{\text{mean}}+(1-\gamma)\vv_e^{\text{iter}}$\\
    Update moving average: $\vv_e^{\text{mean}} \gets detach(\vv_e)$\\
    Correction: $\vv_e \gets \frac{1}{1-\gamma}\vv_e$ (see Appendix \ref{appendix:domainbeddetails})\\
    }

    \uIf{$\text{iter} \geq i_{\text{warmup}}$}{
    Average the domain-level variances: $\vv=\frac{1}{|\mathcal{E}|}\sum_{e\in\mathcal{E}}\vv_{e}$\\
    Compute the regularization loss: $\mathcal{L}_{\text{Fishr}}(\theta)=\frac{1}{|\mathcal{E}|}\sum_{e\in\mathcal{E}}\sum_{\pi\in\omega}|\vv_e^{\pi} - \vv^{\pi}|^2$\\
    $   \mathcal{L}(\theta) \mathrel{{+}{=}} \lambda \mathcal{L}_{\text{Fishr}}(\theta)$
    }
    \tcc{Step 3: gradient descent}%
    Backpropagate gradients: $\theta \gets g\left(\text{gradient}=\nabla_{\theta} \mathcal{L}(\theta), \text{learning rate}=l_r\right)$\\
    }%
    \caption{Training procedure for Fishr on DomainBed}%
    \label{pseudocode}
\end{algorithm}%
