# Supplementary material for: Fishr: Invariant Gradient Variances for Out-of-Distribution Generalization
Source: arXiv:2109.02934 source file (2022-06-01)
Supplement: Supplementary file 2 [file 07_appendix_consistency_iclr.tex]

\subsection{Taylor expansion of the inconsistency score}
\label{appendix:hardtovary}
We further detail the Taylor expansion of the inconsistency score \citep{parascandolo2021learning} used in Section \ref{model:whyhessian}. In the simplified setting $\mathcal{E}=\left\{A,B\right\}$, the inconsistency score goes back to:
$$
\mathcal{I}^{\epsilon}\left(\theta^{*}\right)=\max \left\{\max _{\left|\mathcal{R}_{A}(\theta) - \mathcal{R}_{A}(\theta^{*})\right| \leqslant \epsilon} \left|\mathcal{R}_{B}(\theta) - \mathcal{R}_{A}(\theta^{*})\right|, \max _{\left|\mathcal{R}_{B}(\theta) - \mathcal{R}_{B}(\theta^{*})\right| \leqslant \epsilon} \left|\mathcal{R}_{A}(\theta) - \mathcal{R}_{B}(\theta^{*})\right|\right\} .$$
The second-order Taylor expansion of $\mathcal{R}_{e}$ around $\theta^{*}=0$
(with a change of variable) gives:
$$
\mathcal{R}_{e}(\theta)=\mathcal{R}_{e}(\theta^{*}) + \theta^{\top} \nabla_{\theta} \mathcal{R}_{e}\left(\theta^{*}\right) + \frac{1}{2} \theta^{\top} H_{e} \theta + \mathcal{O}(\left\|\theta\right\|_{2}^2),
$$
for $ e\in\left\{A,B\right\}$. We assume simultaneous convergence, \textit{i.e.}, $\theta^{*}$ is a local minima across all training domains: $\nabla_{\theta} \mathcal{R}_{A}(\theta^{*})=\nabla_{\theta} \mathcal{R}_{B}(\theta^{*})=0$. Thus:
\begin{equation}
\begin{split}
\max _{\left|\mathcal{R}_{A}(\theta) - \mathcal{R}_{A}(\theta^{*})\right| \leqslant \epsilon} \left|\mathcal{R}_{B}(\theta) - \mathcal{R}_{A}(\theta^{*})\right| &\approx \max _{\left|\frac{1}{2} \theta^{\top} H_{A} \theta\right| \leqslant \epsilon} \left|\mathcal{R}_{B}(\theta^{*}) + \frac{1}{2} \theta^{\top} H_{B} \theta - \mathcal{R}_{A}(\theta^{*})\right|\\
&\lessapprox \left|\mathcal{R}_{B}(\theta^{*}) - \mathcal{R}_{A}(\theta^{*})\right| + \max _{\left|\frac{1}{2} \theta^{\top} H_{A} \theta\right| \leqslant \epsilon} \left|\frac{1}{2} \theta^{\top} H_{B} \theta \right|,
\end{split}
\end{equation}
where the last inequality is deduced from the triangle inequality.

The first term $\left|\mathcal{R}_{B}(\theta^{*}) - \mathcal{R}_{A}(\theta^{*})\right|$ was simply assumed small at convergence in AND-mask \citep{parascandolo2021learning}. We further justify this approximation for Fishr by reminding that the empirical risks difference across domains is the V-REx \citep{krueger2020utofdistribution} criterion: thus, as argued in Section \ref{model:fishrmatchgradient} and as shown in Appendix \ref{appendix:fishrrex}, Fishr forces this first term to be low at convergence.
%  $\left|\mathcal{R}_{B}(\theta^{*}) - \mathcal{R}_{A}(\theta^{*})\right|\to 0$ and

% Following \citet{parascandolo2021learning}, the second term is more easily understood when Hessians are diagonal: $\mH_{e}=\operatorname{diag}\left(\lambda_{1}^{e}, \cdots, \lambda_{n}^{e}\right)$ with $\forall i\in \left\{1, \ldots, |\theta|\right\}, \lambda_{i}^{e} > 0$. In this case,
% $\max _{\left|\frac{1}{2} \theta^{\top} H_{A} \theta\right| \leqslant \epsilon} \left|\frac{1}{2} \theta^{\top} H_{B} \theta \right|= \epsilon \cdot \max _{i} \frac{\lambda_{i}^{B}}{\lambda_{i}^{A}}$
% % The result holds when Hessians are co-diagonalizable.
% is large when $\exists i, \lambda_i^A$ is small but $\lambda_i^B$ is large.
% That's why $\mathcal{I}^{\epsilon}\left(\theta^{*}\right)\approx\epsilon \cdot \max _{i} \max \left\{\frac{\lambda_{i}^{B}}{\lambda_{i}^{A}}, \frac{\lambda_{i}^{A}}{\lambda_{i}^{B}}\right\}$ decreases when $\mH_A$ and $\mH_B$ have close eigenvalues.
Following \citet{parascandolo2021learning}, the second term is more easily understood when Hessians are diagonal: $\mH_{e}=\operatorname{diag}\left(\lambda_{1}^{e}, \cdots, \lambda_{n}^{e}\right)$ with $\forall i\in \left\{1, \ldots, |\theta|\right\}, \lambda_{i}^{e} > 0$.
In this case,
$\max _{\left|\frac{1}{2} \theta^{\top} H_{A} \theta\right| \leqslant \epsilon} \left|\frac{1}{2} \theta^{\top} H_{B} \theta \right|=
\max _{\|\tilde{\theta}\|^{2} \leqslant \epsilon} \sum_{i} \tilde{\theta}_{i}^{2} \lambda_{i}^{B}/\lambda_{i}^{A} =
\epsilon \cdot \max _{i} \lambda_{i}^{B}/\lambda_{i}^{A}$
% The result holds when Hessians are co-diagonalizable.
is large when $\exists i$ such that $\lambda_i^A$ is small but $\lambda_i^B$ is large.
Thus, $\mathcal{I}^{\epsilon}\left(\theta^{*}\right)\lessapprox\epsilon \cdot \max  \max _{i} \left\{\lambda_{i}^{B}/\lambda_{i}^{A}, \lambda_{i}^{A}/\lambda_{i}^{B}\right\}$ decreases when $\mH_A$ and $\mH_B$ have similar eigenvalues.

In conclusion, Fishr reduces inconsistency by matching (1) domain-level  empirical risks and (2) domain-level Hessians across the training domains.

% As a reminder,
% $\mathcal{I}^{\epsilon}\left(\theta^{*}\right)=\max_{(e, e^{\prime})\in\mathcal{E}^2} \max_{\theta \in N_{A, \theta^{*}}^{\epsilon}}\left|\mathcal{R}_{e^{\prime}}(\theta)-\mathcal{R}_{e}(\theta^{*})\right|$.


% In conclusion, the inconsistency score is
% $\mathcal{I}^{\epsilon}\left(\theta^{*}\right)\approx\left|\mathcal{R}_{B}(\theta^{*}) - \mathcal{R}_{A}(\theta^{*})\right| + \epsilon \cdot \max _{i} \max \left\{\frac{\lambda_{i}^{B}}{\lambda_{i}^{A}}, \frac{\lambda_{i}^{A}}{\lambda_{i}^{B}}\right\}$ at convergence.
% Both terms are minimized by the Fishr strategy. The first




% This is how, for $\mathcal{E}=\left\{A,B\right\}$ and diagonal (or co-diagonalizable) Hessians $\mH_{e}=\operatorname{diag}\left(\lambda_{1}^{e}, \cdots, \lambda_{n}^{e}\right)$ with $\forall i\in \left\{1, \ldots, |\theta|\right\}, \lambda_{i}^{e} > 0$, they show that:

% \citep{ando2004geometric}
% $\mathcal{I}^{\epsilon}\left(\theta\right) \leqslant 2 \epsilon\left(\frac{\operatorname{det}\left(\mH_{A+B}\right)}{\operatorname{det}\left(\mH_{A \wedge B}\right)}\right)^{2}$ when $\mathcal{E}=\left\{A,B\right\}$.
% $\mathcal{I}^{\epsilon}\left(\theta^{*}\right) \leqslant 2 \epsilon\left(\operatorname{det}\left(\mH_{A+B}\right) / \operatorname{det}\left(\mH_{A \wedge B}\right)\right)^{2}$.
% Similar property holds true when domain-level Hessians are simultaneously .
